# Supplementary material for: Object-centric Forward Modeling for Model Predictive Control
Source: arXiv:1910.03568 source file (2019-10-08)
Supplement: Supplementary file 1 [file main_appendix.tex]

\documentclass{article}

\usepackage{wrapfig}
\usepackage[final]{corl_2019} % Uncomment for the camera-ready ``final'' version
\usepackage[utf8]{inputenc} % allow utf-8 input
\usepackage[T1]{fontenc}    % use 8-bit T1 fonts
\usepackage{url}            % simple URL typesetting
\usepackage{booktabs}       % professional-quality tables
\usepackage{amsfonts}       % blackboard math symbols
\usepackage{amsmath}
\usepackage{amssymb}
\usepackage{nicefrac}       % compact symbols for 1/2, etc.
\usepackage{microtype}      % microtypography
\usepackage{lib}

\usepackage{graphicx}
\usepackage{subfig}
\usepackage[font=footnotesize,labelfont=bf]{caption} % to make caption text small, check if nips likes it.
\usepackage[title]{appendix}

\begin{document}
\title{Supplementary: Object-centric Forward Modeling \\ for  Model Predictive Control}
% \title{Learning Compositional Forward Modeling \\ for Model Predictive Control}
% The \author macro works with any number of authors. There are two
% commands used to separate the names and addresses of multiple
% authors: \And and \AND.
%
% Using \And between authors leaves it to LaTeX to determine where to
% break the lines. Using \AND forces a line break at that point. So,
% if LaTeX puts 3 of 4 authors names on the first line, and the last
% on the second line, try using \AND instead of \And before the third
% author name.

% NOTE: authors will be visible only in the camera-ready (ie, when using the option 'final'). 
% 	For the initial submission the authors will be anonymized.

\author{Yufei Ye\textsuperscript{1}  \qquad Dhiraj Gandhi \textsuperscript{2} \qquad Abhinav Gupta\textsuperscript{12} \qquad Shubham Tulsiani\textsuperscript{2} \\
% \vspace{-2mm}
\textsuperscript{1}Carnegie Mellon University  \qquad \textsuperscript{2}Facebook AI Research \\
{\tt \small yufeiy2@cs.cmu.edu \qquad \{dhirajgandhi,gabhinav,shubhtuls\}@fb.com}
\\
{\tt \small \href{https://judyye.github.io/ocmpc/}{https://judyye.github.io/ocmpc/}}
}

\maketitle

\input{src/appendix.tex}
\end{document}
